# Supplementary material for: SE-GAN: Skeleton Enhanced GAN-based Model for Brush Handwriting Font Generation
Source: arXiv:2204.10484 source file (2022-04-22)
Supplement: Supplementary file 1 [file Appendix.tex]

\section*{Appendix}
In this section, we supplement some extra information and experimental results, which includes: 1) We present the detailed features of collected 6 style of brush handwriting dataset; 2) We explain the methods used for skeleton extraction and present samples of generated skeleton images during experiments; 3) we also explain the experimental setup with detailed information for data processing and model training; 4) we also present the compared results with baselines on SPFG tasks to show the generalisation ability of SE-GAN.

\section{Dataset}
As the deficiency of public brush handwriting font generation dataset, we collect a large-scale image dataset for experiments. As shown in Fig. \ref{fig:dataset}, there are six different chirography styles in total. Each style of fonts are collected from the daily calligraphy practice of a professional calligrapher. It's observed that each chirography style of fonts have their own distinct and impressive features, and some of them are even written in a semi-cursive or cursive way. The corresponding visual features and patterns for each style are also summarized in Fig. \ref{fig:dataset} for better understanding the difficulty of this dataset. The statistics of each style is presented in Table 1 of original paper. During experiements, we split each subset into train/dev/test set by ratio of 8:1:1. We choose the standard print font Liukai as the source domain, and take each of the six styles as the target domain respectively. During data collection, we scan and reform all the images to 1250 $\times$ 1250 pixel resolution. In our experiments, all of images are resized into 256 $\times$ 256 pixel for model training.  

\section{Skeleton Extraction}
\label{sect:selection}
In general, skeleton contains the basic information of character, such as the composition and position of strokes, writing direction, etc. It represent the internal structure and content of a Chinese character, which consists of a collection of thin arcs and curves. As analyzed in the paper, for the same character with different styles, the stylized images should share the same content and structure, which ensure the character images are recognisable. Inspired by \cite{fastthining1984}, we adopt an simple but effective skeletonization algorithm to extract the skeleton image by eroding and dilating the binarized character image iteratively. 
In detail, the binary digitised picture is defied by a matrix $IT$ where each pixel $IT(i,j)$ is either 1 or 0. Iterative transformations are applied to matrix $IT$ point by point according to the values of a small set of neighbouring points. Here we assign $IT$ as $3 \times 3 $ matrix. For efficiency, we adopt parallel processing approach, and the value to be assigned to a point at iteration $t$ depends on the value of eight neighbours at last iteration $t-1$ and its own value on the current time step. This enables the picture to be processed simultaneously and requires only simple computation. 
\begin{figure}[t]
	\centering 
	\includegraphics[width=0.8\linewidth]{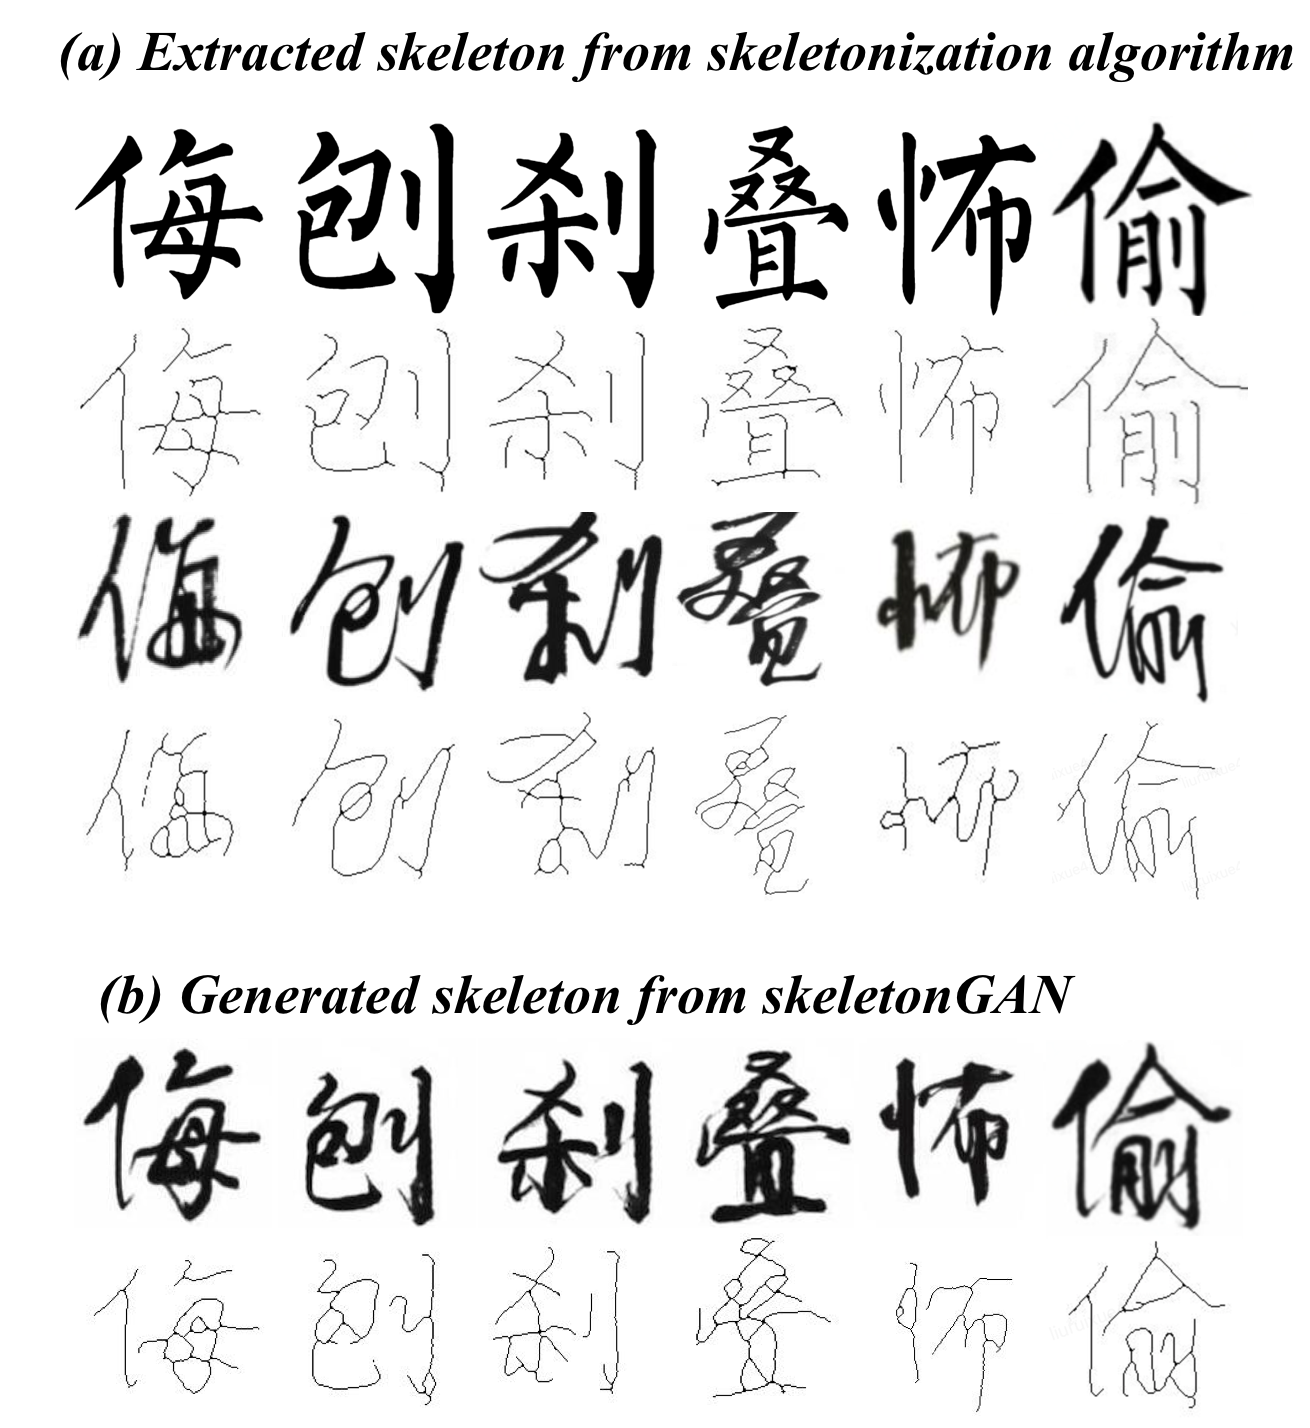}
	\caption{Examples of Extracted and Generated Skeletons.}  
	\label{fig:skeleton}   
\end{figure}
Considering the contribution of skeleton in our proposed model, the performance of skeleton extraction and skeletonGAN also become critical. Here, we demonstrate some skeleton images extracted by the skeletonization algorithm mentioned above and the images generated by the skeletonGAN. Fig. \ref{fig:skeleton} shows that both two approaches can generate very high-quality skeleton images, which indicates the skeleton information plugged in our model is reliable.
Samples of character images and their extracted skeletons are illustrated in Fig. \ref{fig:skeleton}.

\begin{figure*}[htb]
	\centering 
	\includegraphics[width=1\linewidth]{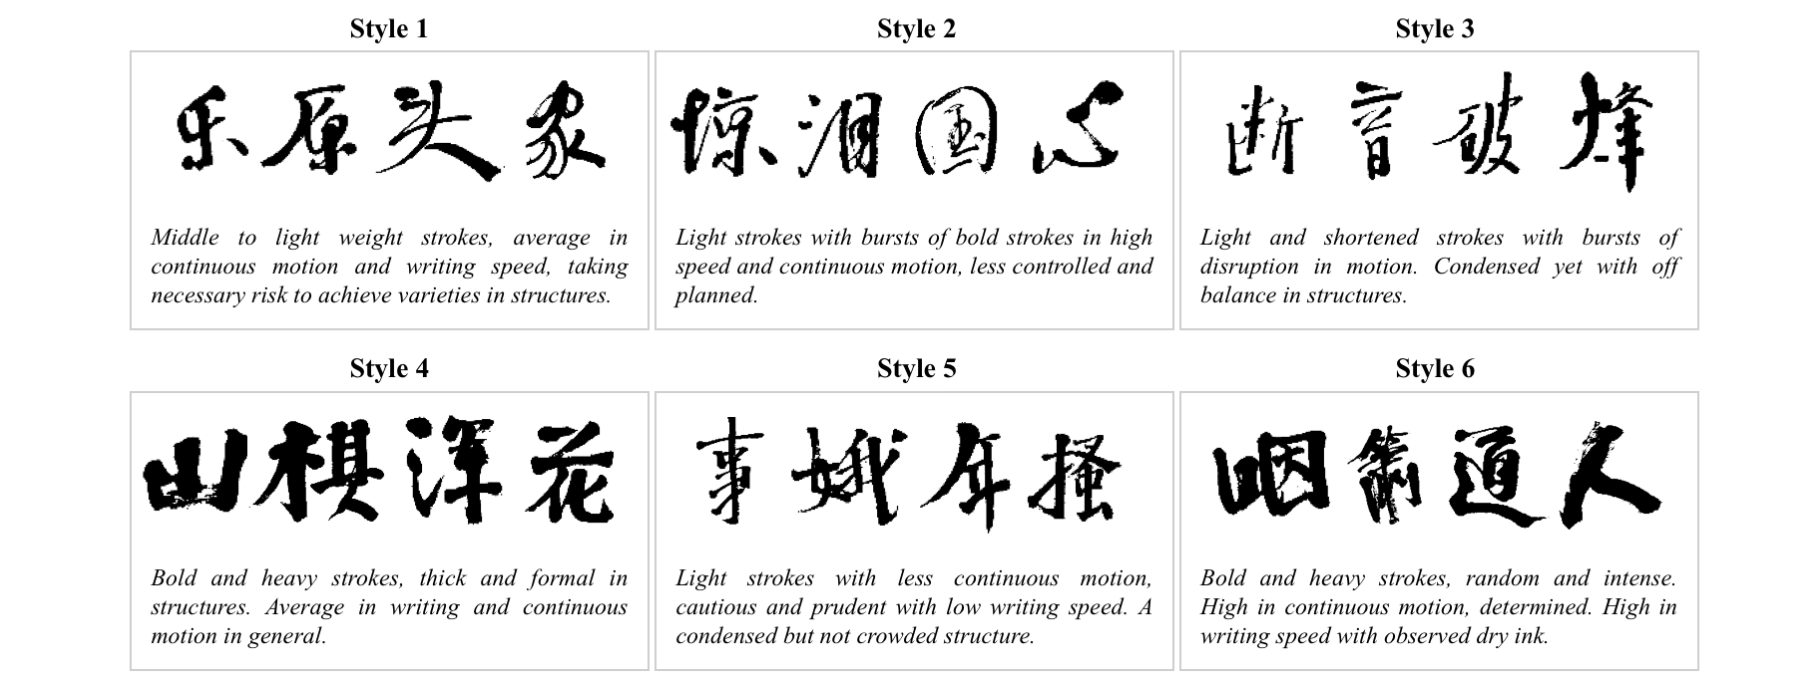}
	\caption{Examples and style descriptions of brush handwriting fonts in our dataset. 
	}
	\label{fig:dataset}   
\end{figure*}
\section{Experimental Setup}
To train the skeletonGAN, we firstly extract the skeleton images of all the characters involved in the experiments with the skeletonization algorithm described in Section \ref{sect:selection}. Then 6000 character images and their corresponding skeleton images are randomly selected for training the CycleGAN \cite{zhu2017cyclegan} model. We train the model for 80 epochs with batch-size of 1. To evaluate the performance of generated skeleton, FID score is calculated. We get a low score of 30.421 on 300 test images. The Low FID score indicates that the pre-trained skeletonGAN is capable of generating high-quality skeleton images.

For image prepossessing, we resize all images to 256 $\times$ 256 pixels and randomly flip them during training for data augmentation. We use Adam optimizer \cite{adam2014} with batch size of 1 and train 100 epochs. In Equation \ref{equt:loss} we set $\lambda_1$=5, 
$\lambda_2$=10, $\lambda_3$=100, and $\lambda_4$=10. For learning rate, we initial it with 0.0001 for the first 8 epoch and then linearly decay it every 5 epochs. All the models are trained on NVIDIA Tesla P40 GPUs.

\section{Experiments on SPFG Task}
%As mentioned before, out model is suitable to handle distinct changes for Chinese characters. Apart from handwritten characters, it's necessary to explore how SE-GAN performs on the standard print font generation task. 
In this section, we are trying to verify if our proposed model will work on the standard print font generation task. We conduct experiments on the popular Sushi font\footnote{
\url{https://www.foundertype.com/index.php/FontInfo/index/id/5001}}. 2400 unpaired images from Liukai and Sushi font library are selected as source and target images respectively for training and 386 images are chosen for testing. Table \ref{table:sushi} illustrates that, compared with CycleGAN and StarGANv2, SE-GAN still has competitive advantage even in SPFG task. And the content accuracy of SE-GAN is close to the upper limit of ground-truth images. Our model also achieves the lowest FID score, which indicates the style of our generated images is close to the target domain.  Fig. \ref{fig:sushi} demonstrates more detailed information for the generated images. The experiment results further prove the generalisation ability of our proposed framework for SPFG task.
\begin{figure}[t]
	\centering 
	\includegraphics[width=0.95\linewidth]{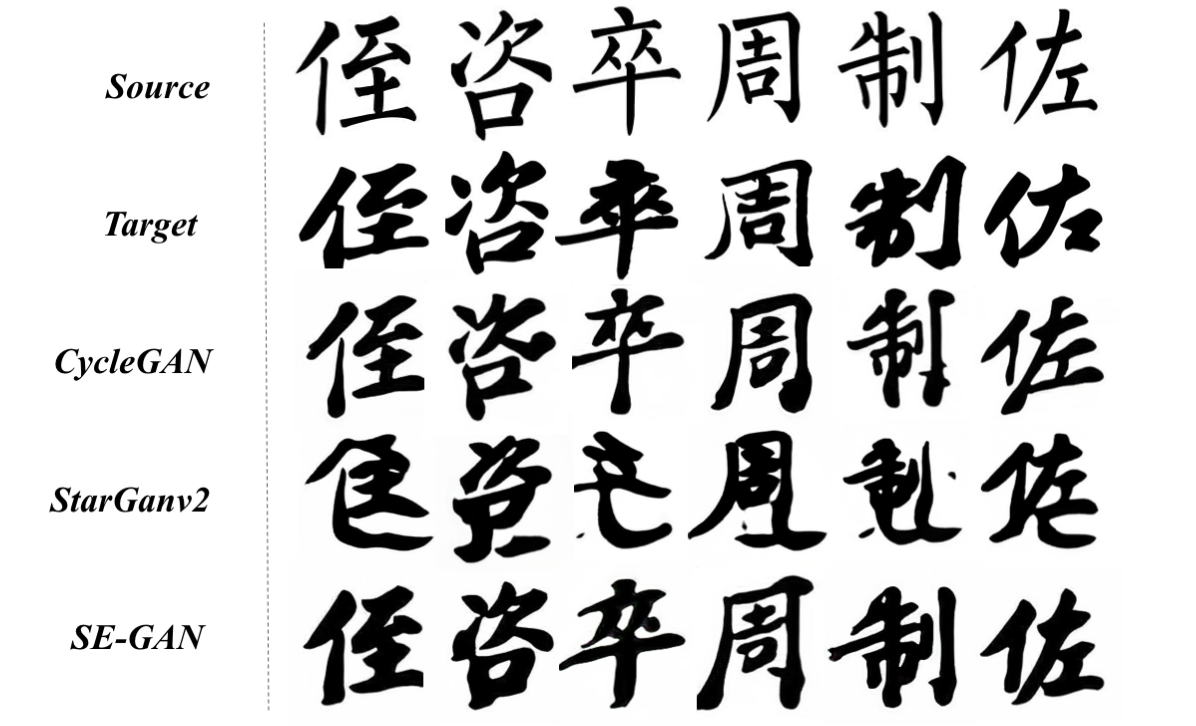}
	\caption{Examples of SPFG (Sushi Font).}  
	\label{fig:sushi}   
\end{figure}

\begin{table}[hb]
\small
\caption{Evaluation results on Sushi Font.}
\centering
\begin{tabular}{l|ccc}
  \hline
  Models & Top1-acc & FID \\ \hline
  CycleGAN & 0.378 & 73.79  \\ 
  StarGANv2 & 0.361 &  70.12 \\ 
  Ours & \textbf{0.582} & \textbf{45.15} \\
  Human & 0.621 & -- \\
  \hline
\end{tabular}
\label{table:sushi}
\end{table}
